# Supplementary material for: $PC^2$: Projection-Conditioned Point Cloud Diffusion for Single-Image 3D Reconstruction
Source: arXiv:2302.10668 source file (2023-02-23)
Supplement: Supplementary file 1 [file 6-appendix.tex]

\section{Implementation Details}\label{s:supplement_implementation}

Here, we provide details about the model and projection procedure which were omitted from the main paper due to space constraints. 

First, we discuss the Point-Voxel~\cite{liu2019pvcnn} model which is used to process the partially-denoised point cloud at each step of the diffusion process. As its name suggests, this model processes a point cloud using two branches simultaneously: a point-based branch and voxel-based branch. The point-based branch is a simple multi-layer perceptron which is applied to each point independently, as in PointNet~\cite{qi2017pointnet,qi2017pointnetpp} (without the global pooling in the final layer of PointNet). The voxel-based branch first discretizes the points into a coarse voxel grid of size $128^3$, which is fed into a 3D U-Net. As in \cite{liu2019pvcnn}, the 3D U-Net consists of four downsampling (``Set Abstraction'') layers followed by four upsampling (``Feature Propogation'') layers. Due to this fine-to-coarse-to-fine structure, the network is able to capture both global and local shape information. Additionally, to make the model aware of the current timestep of the diffusion process, we concatenate an embedding of the current timestep to the point features at the input to each layer.

Second, we discuss the implementation of the projection feature. We perform the projection by rasterizing the point cloud from the given camera view. We utilize the \texttt{PointRasterizer} class of PyTorch3D using a point radius of $0.0075$ and $1$ point per pixel. For each point in the point cloud, if the point is rasterized onto a pixel in the input image, we concatenate the $RGB$ values of the pixel onto that point's existing feature vector (which is simply its current position) for input to the model. Additionally, we concatenate the value of the (binary) object mask at the given pixel and a two-dimensional vector pointing from the pixel to the closest pixel in the mask (i.e. a two-dimensional distance function corresponding to the mask region; this is the zero vector inside the mask and a nonzero vector outside the mask). If a pixel is not rasterized to a point (for example, because it is occluded by another point), we concatenate a vector of zeros in place of all the quantities above. 

\section{Additional Qualitative Examples}\label{s:supplement_qualitative}

We provide additional qualitative examples of our method in \cref{fig:supp_examples_best_1}, \cref{fig:supp_examples_random_1}, and \cref{fig:supp_examples_worst_2}. \cref{fig:supp_examples_best_1} contains a selection of the best reconstructions produced by our model for each category, as ranked by F-score. \cref{fig:supp_examples_random_1} contains random examples of reconstructions produced by our model. Finally, \cref{fig:supp_examples_worst_2} shows a selection of the worst examples produced by our model for each category, as ranked by F-score. 

\section{Analysis of Failure Cases}\label{s:supplement_failure_ases}

As stated above, failure cases of our model are shown in \cref{fig:supp_examples_worst_2}. Examining these failure cases, we observed that our model sometimes performs poorly on images with ambiguous silhouettes/masks. For example, in the $8^{th}$ column of the $2^{nd}$ row of the figure, it appears that the model generated a chair rather than a box. Similarly, in the $12^{th}$ row of the $5^{th}$ row of the figure, the object seems to have generated a box rather than a couch. These errors are most likely due to the fact that these categories all have rectangular silhouettes and shapes which resemble rectangular prisms. 

It is also notable that on many of the challenging examples on which our model struggles (\eg, the examples for the \texttt{watercraft} category located in the last row of the figure), the voxel-based models struggle to a similar degree. 

\section{Interactive Examples of Generated Point Clouds}\label{s:supplement_examples_for_reviewers}

It is difficult to communicate the visual quality of a 3D shape when one is constrained to showing 2D images, as we are in this PDF. Therefore, for the benefit of the reviewers, we have also included a number of interactive examples of point clouds generated by our model in the supplemental material \texttt{zip} file. These are point clouds plotted using the Plotly library and stored as HTML files, so it should be possible to view them interactively on any device with a web browser. For each category in the ShapeNet dataset, we provide three visualization files: (1) an example ground truth mesh, (2) the ground truth point cloud sampled from the mesh, and (3) the reconstructed point cloud generated by our model. 

\section{Comparison with Global Conditioning}\label{s:supplement_global_conditioning}

Here, we provide a small quantitative comparison with a global conditioning approach. In the global conditioning approach, the input image is first processed using a frozen pretrained network (VGG-16~\cite{simonyan2014very}) followed by two learned convolutional layers. The resulting features are pooled into a single vector of size $64$, which is appended to every point at each step of the diffusion process before the point cloud is processed by our network. 

We present results on the airplane and table classes, as these were the primary classes we used while exploring methods during the initial phases of our research. We observed that the globally-conditioned model often produced samples which were reasonable shapes, but which did not match the input images. These results are substantiated by the following table, which shows that the $F$-scores obtained using global conditioning are substantially worse than those obtained using our method: 

\begin{table}[h!]
\label{tab:supplement_comparison_global}
\centering

\begin{tabular}{lccc}
\toprule
\textit{Category} &  Global Cond. & \textbf{\methodname} \\ \midrule
airplane    & 0.197 & \textbf{0.473} \\
table       & 0.156 & \textbf{0.290} \\
\bottomrule
\end{tabular}

\end{table}
